# Supplementary material for: Sociotechnical Harms of Algorithmic Systems: Scoping a Taxonomy for Harm Reduction
Source: arXiv:2210.05791 source file (2023-07-19)
Supplement: Supplementary file 1 [file appendix.tex]

\newpage
\onecolumn
\section{Supplementary Methods}
\label{sec:supplementary_methods}

\subsection{Overview of the Harm Framework}
\label{harmframework}
\begin{table}[ht]
\fontsize{7.2}{8.2}\selectfont
\centering
\setlength{\tabcolsep}{4.5pt}
\caption{Sociotechnical harm framework with specific harm types}
\resizebox*{\linewidth}{!}{
\begin{tabular}{p{2cm}p{4cm}p{10.5cm}}

\toprule
Harm Theme & Sub-Types & Specific Harms \\ \midrule
Representational & Stereotyping & Oversimplified and undesirable representations \\  \cline{2-3}
 & Demeaning social groups & Representations of a particular group as a lower social status using discourses, images, and language used to marginalize or oppress a social group \\  \cline{2-3}
 & Erasing social groups & Hegemonic ideas or social relations normalized in algorithmic systems \\ 
 &  & Systemic illegibility or absence of social groups in algorithmic system inputs/outputs \\ 
 &  & Unequal visibility of certain social groups \\  \cline{2-3}
 & Alienating social groups & Failure to acknowledge one’s membership in a culturally significant social group \\
 &  & Classifying or describing socially significant events in ways that ignores social injustices \\  \cline{2-3}
 & Denying opportunity to self-identify & Non-consensual classifications or representations of a person in algorithmic systems \\  \cline{2-3}
 & Reifying essentialist social \par categories & Reinforcing socially constructed categories as ‘natural’ \\  \hline
Allocative & Opportunity loss & Discrimination in critical resource domains (e.g., education, government, healthcare, or housing) \\
 &  & Inequitable access to resources needed to equitably participate in society \\  \cline{2-3}
 & Economic loss & Employment or hiring discrimination \\
 &  & Demonetization based on sensitive characteristics \\
 &  & Discrimination in  insurance, banking, or other financial sectors \\  
 &  & Financial losses or injuries, including price   discrimination \\  \hline
Quality-of-service & Alienation & Adverse emotions (e.g., frustration, bother, disappointment, or anger) experienced when interacting with technologies that fail based on one’s identity characteristics \\
 &  & Algorithmic invisibility, or feelings of exclusion from using non-inclusive technologies \\ \cline{2-3}
 & Increased labor & Additional effort required to make technologies operate as intended \\
 &  & Identity-based accommodation   to technologies (e.g., linguistic) \\
 &  & Wasted time/labor based on technology failures \\\cline{2-3}
 & Service or benefit loss & Degraded performance based on identity characteristics \\
 &  & Disproportionate loss of technological benefits \\ \hline
Interpersonal & Loss of agency or control & Algorithmically-informed identity change \\
 &  & Algorithmic profiling \\
 &  & Loss of autonomy \\
 &  & Required use of specific technologies to access domains that affect material well-being \\  \cline{2-3}
 & Tech-facilitated violence & Coercive control, or intimate partner violence \\
 &  & Device lockout and control \\
 &  & Inciting or enabling offline violence \\
 &  & Online abuse (e.g., cyberbullying, deadnaming, doxxing, trolling, hateful or toxic language, gender-based sexual harassment) \\  \cline{2-3}
 & Diminished health/well-being & Behavioral manipulation \\
 &  & Emotional harms (e.g., dignity loss, invalidation, misgendering, psychological harms) \\
 &  & Physical harms \\
 &  & Reputational harms \\  \cline{2-3}
 & Privacy violations & Exploitative or undesired inferences \\
 &  & Feelings of surveillance, or loss of desired anonymity \\
 &  & Loss of right to be forgotten \\
 &  & Non-consensual data collection \\
 &  & Privacy attacks (e.g., identity theft, doxxing) \\ \hline
Social/societal & Information harms & Disinformation \\
 &  & Distortion of reality (e.g., creation of information “bubbles”) \\
 &  & Malinformation \\
 &  & Misinformation \\
 &  & Subjugating knowledges or foreclosing alternative ways of knowing \\  \cline{2-3}
 & Cultural harms & Cultural hegemony \\
 &  & Deteriorating social bonds \\
 &  & Proliferating false perceptions about cultural groups \\
 &  & Systemic erasure of culturally significant objects and practices \\  \cline{2-3}
 & Political and civic harms & Erosion of democracy (e.g., election interference, censorship, harm to civil liberties) \\
 &  & Human rights violations \\
 &  & Legal system harms (e.g., wrongful arrest, court   transcription errors, unreasonable searches) \\
 &  & Nation destabilization (e.g., social   polarization, loss of legitimacy) \\  \cline{2-3}
 & Macro socio-economic harms & Digital divides \\
 &  & Labor exploitation \\
 &  & Systemic failures of financial systems \\
 &  & Technological unemployment (e.g., deskilling,   devaluation of human labor, or job displacement) \\  \cline{2-3}
 & Environmental harms & Damage to natural environment \\
 &  & Damage to built environment or property \\
 &  & Depletion or contamination of natural resources \\
 &  & Injury to animals \\ \hline
\end{tabular}}
\end{table}

\subsection{Composition of the Corpus}
Here, we first provide additional detail of the corpus identified discussed in the Methods Section \ref{methods} on data collection, descriptive statistics of the corpus, and data sources. Then in Section \ref{harmframework} we present a high level overview of the harms framework.
\subsubsection{Data collection} 
 The corpus contains 172 papers published across the 12-year span surveyed. Our data collection aligns to prior systematic reviews in computing literature, in accordance with the Preferred Reporting Items for Systematic Reviews and Meta-Analyses (PRISMA). Figure \ref{fig:Prisma} illustrates the adapted PRISMA flowchart detailing the data collection process for inclusion in the corpus.

 \begin{figure}[!ht]
    \centering
     \caption{PRISMA flow diagram.}
    \label{fig:Prisma}
    \includegraphics[width=1\textwidth]{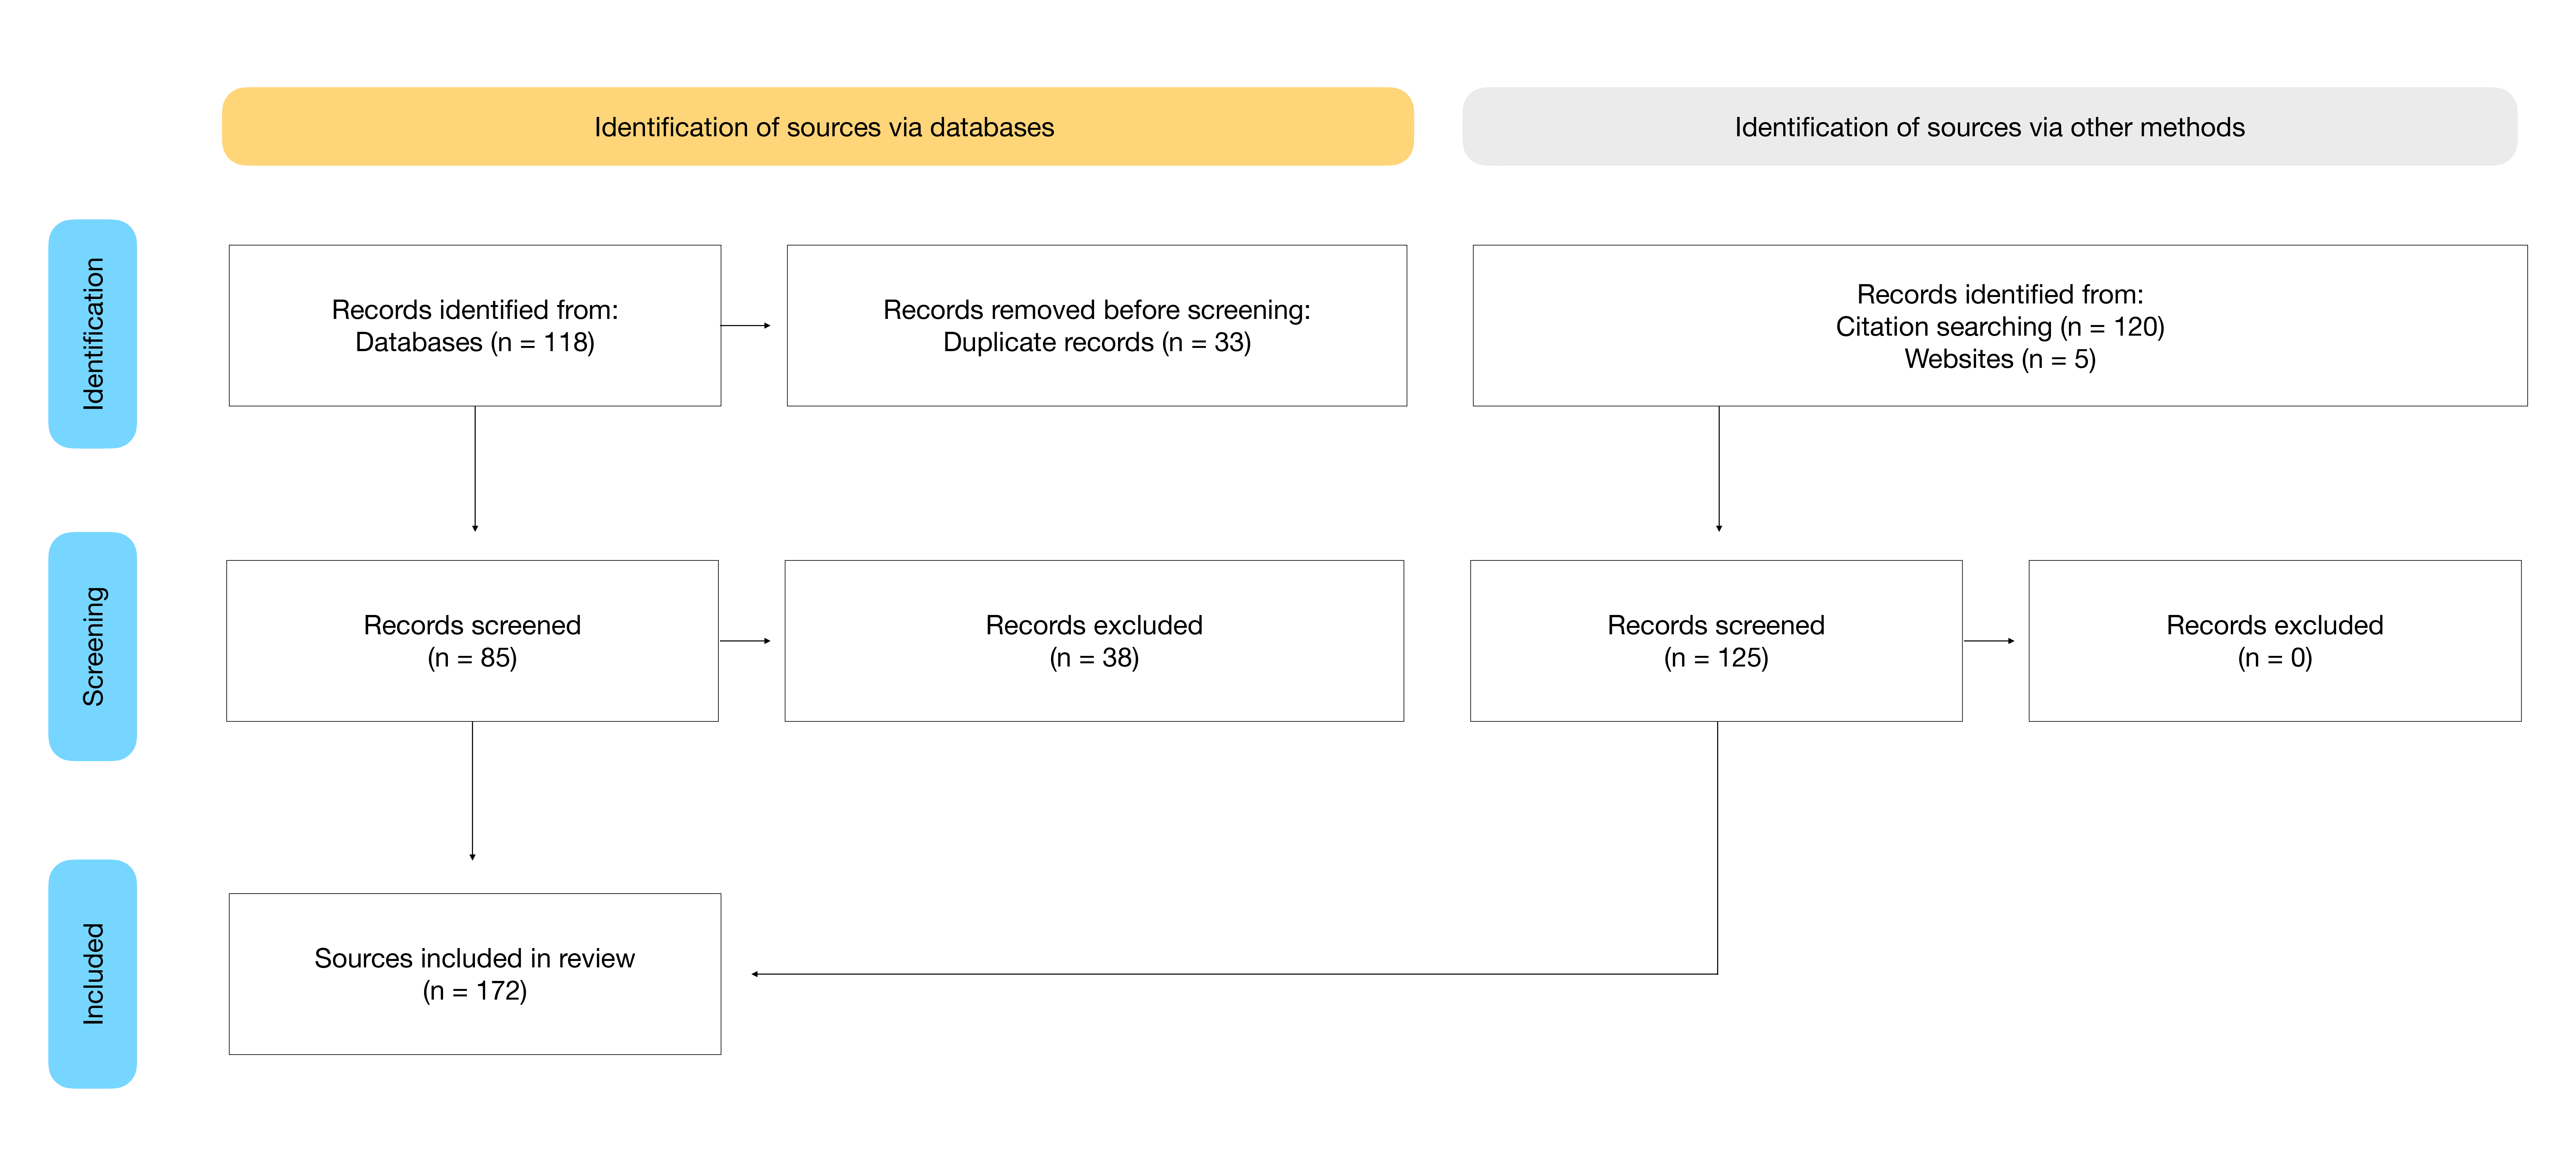}
\end{figure}

\subsubsection{Excluded sources} The initial search of the ACM database produced a set of 85 research articles (duplicates removed from 118 papers). The citations-based review and targeted keyword searches of NGO and professional organization outputs identified an additional 125 resources. We included articles that described or discussed: (1) algorithmic technologies and (2) harms or adverse impacts from algorithmic systems. We excluded 38 articles that: (1) did not meet the inclusion criteria, and (2) did not have full-text available. In total, 172 articles and frameworks were included in our corpus. Table \ref{Excluded sources} summarizes excluded sources.

\subsubsection{Publication year} A little over two-thirds (\textit{n}=17, 68\%) of them have been published in the last three years (2020–2022). Figure \ref{fig:figure1} provides the distribution of papers by year, while Figure \ref{fig:figure2} provides the distribution by sociotechnical harm type. Though Figure \ref{fig:figure2} captures a widening range of different harm types, we urge readers to recognize harms as overlapping and multidimensional.

\subsubsection{Publication venue} The corpus is comprised of literature from academic conferences (\textit{n}=81, 47\%), scholarly journals (\textit{n}=56, 32\%), and gray literature (\textit{n}=35, 20\%). Within academic conferences, approximately 91\% of articles were published in ACM venues, including the ACM CHI Conference (\textit{n}=22, 27\%), ACM FAccT Conference (\textit{n}=21, 26\%), ACM CSCW Conference (\textit{n}=9, 11\%), AAAI/ACM Conference on AI, Ethics, and Society (\textit{n}=7, 8\%). Of research published in scholarly journals, venues varied widely, including ACM and IEEE publications, and key field journals such as \textit{Big Data \& Society}, \textit{Social Media + Society}, and \textit{Nature Machine Intelligence}. Of gray literature, three-quarters of articles were preprints published on arXiv (70\%) and the Social Science Research Network (5\%).

\begin{figure}[!ht]
  \centering
  \caption{Number of articles (y axis) included in the corpus by publication year (x axis)}
  \includegraphics[width=.8\textwidth]{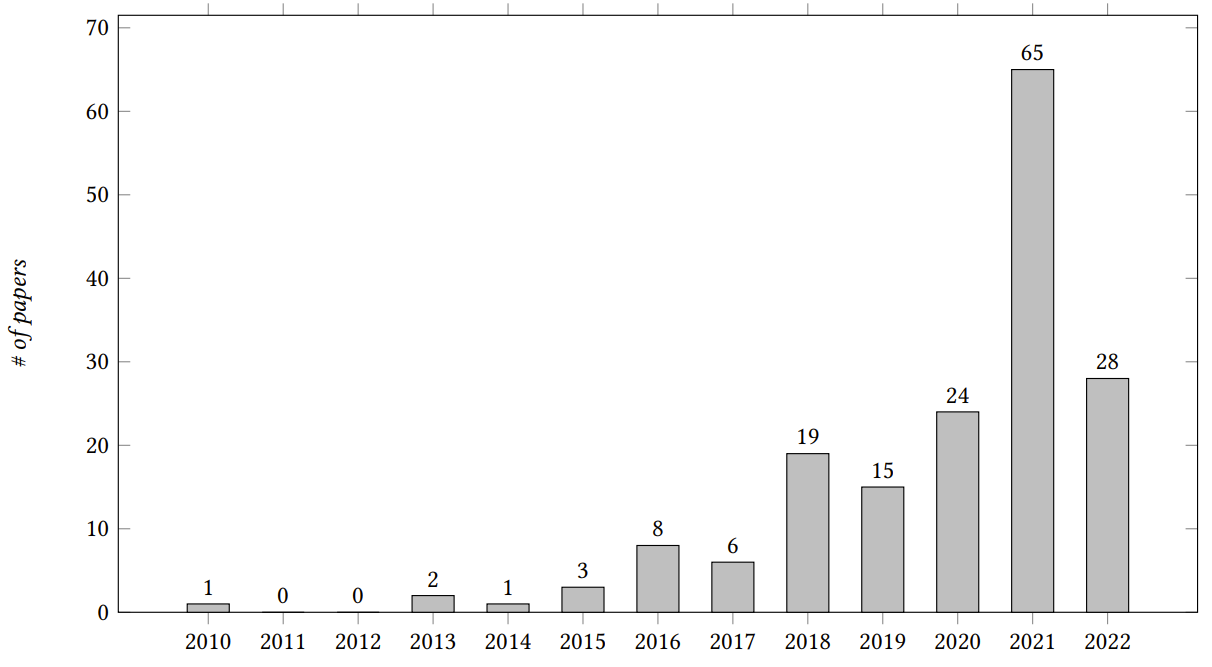}
  \label{fig:figure1}
\end{figure}

\begin{figure}[!ht]
  \centering
  \caption{Percentage plot of papers coded by year (x axis) and for each harm type (y axis)}
  \includegraphics[width=.9\textwidth]{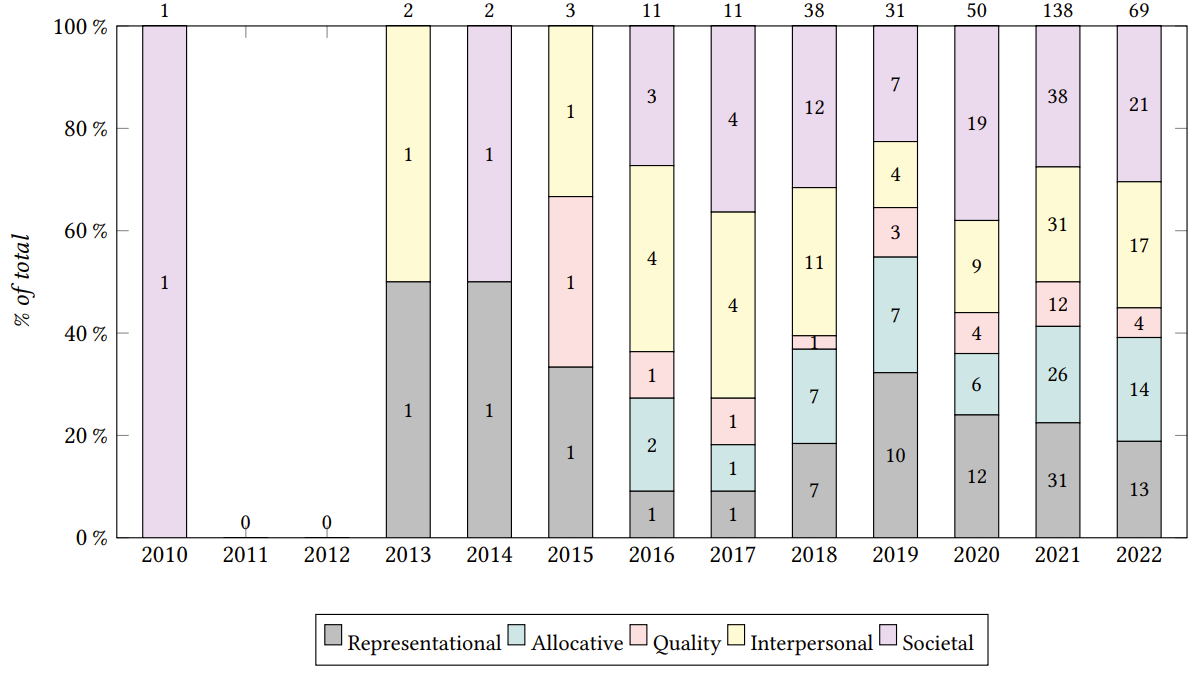}
  \label{fig:figure2}
\end{figure}

\newpage
%\vspace{10mm}
\newpage
%\begin{center}
\begin{longtable}{@{} p{.75cm}p{4.5cm}p{7.5cm}p{3cm}}
\caption{Excluded sources.}
\label{Excluded sources}
\\
\toprule
Year & Author(s) & Title & Reason for Exclusion \\ \midrule
1993 & Kernohan, A. & Accumulative Harms and the Interpretation of the Harm Principle & Does not describe algorithmic systems \\ \hline
2008 & Klaus-Dieter, S., \& Thalheim, B. & Storyboarding Concepts for Edutainment WIS & Not focused on algorithmic system harms \\ \hline
2016 & Fiesler, C., Wisniewski, P., Pater, J., \& Andalibi, N. & Exploring Ethics and Obligations for Studying Digital Communities & Call for papers \\ \hline
2018 & Garvey, C. & AI Risk Mitigation Through Democratic Governance: Introducing the  7-Dimensional AI Risk Horizon & Full-text not available \\ \hline
2018 & Walker, W. & "Data Justice" By Design: Building Engagement Through Civic Technologies & Full-text not available \\ \hline
2018 & Passi, S., \& Jackson, S.J. & Trust in Data Science: Collaboration, Translation, and Accountability in Corporate Data Science Projects & Not focused on algorithmic system harms \\ \hline
2018 & Veale, M., Van Kleek, M., \& Binns, R. & Fairness and Accountability Design Needs for Algorithmic Support in High-Stakes Public Sector Decision-Making & Not focused on algorithmic system harms \\ \hline
2019 & Rempel, E., Barnett, J., \& Durrant, H. & Contrasting Views of Public Engagement on Local Government Data Use in the UK & Not focused on algorithmic system harms \\ \hline
2019 & Ekstrand, M.D., Burke, R., \& Diaz, F. & Fairness and Discrimination in Recommendation and Retrieval in RecSys ‘19 & Full-text not available \\ \hline
2019 & Ekstrand, M.D., Burke, R., \& Diaz, F. & Fairness and Discrimination in Recommendation and Retrieval in SIGIR ‘19 & Full-text not available \\ \hline
2020 & Cath, C., Latonero, M., Marda, V., \& Pakzad, R. & Leap of FATE: Human Rights as a Complementary Framework for AI Policy and Practice & Conference tutorial \\ \hline
2020 & Dias, V., Lokanathan, S., \& Wijeratne, Y. & A Brief Primer on Bias in Machine Learning and Algorithmic Decisions [White Paper] & Full-text source available is incomplete \\ \hline
2020 & Theodorou, A., \& Dignum, V. & Towards Ethical and Socio-legal Governance in AI. & Full-text source unavailable \\ \hline
2020 & Baker, D., Hanna, A., \& Denton, E. & Algorithmically Encoded Identities: Reframing Human Classification & Full-text source unavailable \\ \hline 
2020 & Jacobs, A.Z., Blodgett, S.L., Barocas, S., Daumé, H., \& Wallach, H. & The Meaning and Measurement of Bias: Lessons from Natural Language Processing & Conference tutorial \\ \hline
2020 & Zhuang, W., Wen, Y., Zhang, X., Gan, X., Yin, D., Zhou, D., Zhang, S., \& Yi, S. & Performance Optimization of Federated Person Re-identification via Benchmark Analysis & Not focused on algorithmic system harms \\ \hline
2021 & Metaxa, D., Park, J., Robertson, R., Karahalios, K., Wilson, C., Hancock, J., \& Sandvig, C. & Auditing Algorithms: Understanding Algorithmic Systems from the Outside In & Focused on machine behaviors, rather than harms \\ \hline
2021 & Watkins, E., Moss, E., Metcalf, J., Singh, R., \& Elish, M. & Governing Algorithmic Systems with Impact Assessments: Six Observations & Focused on Impact Assessments \\ \hline
2021 & Zhou, F., Yu, L., Xu, X., \& Trajcevski, G. & Decoupling Representation and Regressor for Long-Tailed Information Cascade Prediction & Focused on harm to models, rather than harms from models \\ \hline
2021 & Hanna, J.P., Niekum, S., \& Stone, P. & Importance Sampling in Reinforcement Learning with an Estimated Behavior Policy & Not focused on algorithmic system harms \\ \hline
2021 & Whittaker, M. & The Steep Cost of Capture & Not focused on harms from algorithmic systems \\ \hline
2021 & Gaikwad, S.N., Iyer, S., Lunga, D., \& Bondi, E. & Data-driven Humanitarian Mapping: Harnessing Human-Machine Intelligence for High-Stake Public Policy and Resilience Planning & Full-text not available \\ \hline
2021 & Benitez, Y.S. & Algorithmic Ecologies of Justice: Using Computational Social Science Methods to Co-design Tools of Resistance, Resilience and Care with Communities & Full-text not available \\ \hline
2022 & Birhane, A., Kalluri, P., Card, D., Agnew, W., Dotan, R., \& Bao, M. & The Values Encoded in Machine Learning Research & Not focused on algorithmic system harms \\ \hline
2022 & Abdellatif, A., Mhaisen, N., Mohamed, A., Erbad, A., Guizani, M., Dawy, Z., \& Nasreddine, W. & Communication-efficient Hierarchical Federated Learning for IoT Heterogeneous Systems with Imbalanced Data & Not focused on algorithmic system harms \\ \hline
2022 & Shah, C., Suel, T., Diaz, F., Mitra, B., Poblete, B., Suleman, H., \& Verberne, S. &
Report on the 44th International ACM SIGIR Conference on Research and Development in Information Retrieval & Not focused on algorithmic system harms \\ \hline
2022 & Berridge, C., Zhou, Y., Lazar, A., Porwal, A., Mattek, N., Gothard, S., \& Kaye, J. &
Control Matters in Elder Care Technology: Evidence and Direction for Designing IT & Not focused on algorithmic system harms \\ \hline
2022 & Olewicki, D., Nayrolles, M., \& Adams, B. & Towards Language-independent Brown Build Detection & Focused on harm to models, rather than harms from models \\ \hline
2022 & Hamed, I., Denisov, P., Li, C., Elmahdy, M., Abdennadher, S., \& Vu, N. & Investigations on Speech Recognition Systems for Low-resource Dialectal Arabic–English Code-switching Speech & Not focused on algorithmic system harms \\ \hline
2022 & Lum, K., Zhang, Y., \& Bower, A. & De-biasing “Bias” Measurement & Not focused on algorithmic system harms \\ \hline
2022 & Zhang, L., Lu, X., Chen, Z., Liu, T., Chen, Q., \& Li, Z. & Adaptive Deep Learning for Network Intrusion Detection by Risk Analysis & Not focused on algorithmic system harms \\ \hline
2022 & Young, M., Katell, M., \& Krafft, P.M. & Confronting Power and Corporate Capture at the FAccT Conference & Not focused on algorithmic system harms \\ \hline
2022 & Howard, N., Madkins, T., \& White, S.V. & Disrupting Anti-Blackness While Making Room for Black Girls and Women in CS and Tech & Full-text not available \\ \hline
2022 & Blodgett, S.L., Liao, Q.V., Olteanu, A., Mihalcea, R., Muller, M., Scheuerman, M.K., Tan, C., \& Yang, Q. & Responsible Language Technologies: Foreseeing and Mitigating Harms & Full-text not available \\ \hline
2022 & Li, Z., Nie, J., Song, Y., Du, P., \& Li, D. & Learning to Classify Relations Between Entities from Noisy Data - A Meta-Instance Reweighting Approach & Not focused on algorithmic system harms
\end{longtable}
%\end{center}

\newpage
\subsection{Data Sources}
The tables in this section provide references for each harm type and sub-type included in the corpus. %As some sources referenced multiple types and sub-types of harm, they appear several times.

%\newpage
\begin{center}
\begin{longtable}{p{5cm}p{8cm}}
\caption{Representational harms described in data sources.}
\label{representationaldatasources}\\
\toprule
Sub-type & References \\ \midrule
%\endfirsthead
%\toprule
%Harm Theme & Instances & References \\ \midrule
%\endhead 
%\endfoot
%\bottomrule 
%\endlastfoot
Representational harms (generally) &  \cite{Andalibi_Garcia_2021, Bailey_Burkell_Dunn_Gosse_Steeves_2021, Balayn_Lofi_Houben_2021, Bandy2021, Barabas_Doyle, barocas-hardt-narayanan, Bengio_Beygelzimer_Crawford_Fromer_Gabriel_Levendowski_Raji_Ranzato_2022, Birhane_Prabhu_Kahembwe_2021, Blodgett_Barocas_Daume_Wallach_2020, Castillo_2019, Chi_Lurie_Mulligan,corry2021problem, Davis_Williams_Yang_2021, DeVos_Dhabalia_Shen_Holstein_Eslami_2022, Dobbe_Dean_Gilbert_Kohli_2018, Ekstrand_Das_Burke_Diaz_2022, galaz2021artificial, galaz2021machine, Hendricks_Burns_Saenko_Darrell_Rohrbach_2018, Holstein_2019, Hutchinson_Prabhakaran_Denton_2020, Jane_2018, Karizat_2021, Katzman_Barocas_Blodgett_Laird_Scheuerman_Wallach_2021, Kay_Matuszek_Munson_2015, Knox_2019, Lloyd_2018, Luccioni_Corry_Sridharan_Ananny_Schultz_Crawford_2022, Mannes_2020, Markl_2022, Mashhadi_Zolyomi_Quedado_2022, Monroe-White_2021, Paullada_Raji_Bender_Denton_Hanna_2021,  Pruksachatkun_Krishna_Dhamala_Gupta_Chang_2021,Richardson_Gilbert_2021, Rincon_Keyes_Cath_2021, Savoldi_Gaido_Bentivogli_Negri_Turchi_2021, Sun_Asudeh_Jagadish_Howe_Stoyanovich_2019, Sweeney_2013, vanEs_2021, Wang_Barocas_Laird_Wallach_2022, Weidinger2022, Weinberg_2022, Wu_Mitra_Ma_Diaz_Liu_2022, Yee_Tantipongpipat_Mishra_2021, Zajko_2022, Zhao_Wang_Yatskar_Ordonez_Chang_2017, binns2021, dacon2021does, rekabsaz2021, Chancellor_2019, Hutchinson2020socialbiases, phan2019amazon, Moore2020, Marda_Narayan_2020, tomalin2021practical, Tantipongpipat2019, samadi2018, BarocasSelbst_2016}  \\ \midrule
Stereotyping social groups & \cite{Abid_Farooqi_Zou_2021, Balayn_Lofi_Houben_2021, Bandy2021, binns2021, Birhane_Prabhu_Kahembwe_2021, Blodgett_Barocas_Daume_Wallach_2020, Cambre_Kulkarni_2019, Davis_Williams_Yang_2021, DeVos_Dhabalia_Shen_Holstein_Eslami_2022, Dev_Monajatipoor_Ovalle_Subramonian_Phillips_Chang_2021, Dobbe_Dean_Gilbert_Kohli_2018, Hendricks_Burns_Saenko_Darrell_Rohrbach_2018, Hutchinson_Prabhakaran_Denton_2020, Kaminski_Malgieri_2020, Katzman_Barocas_Blodgett_Laird_Scheuerman_Wallach_2021, Kay_Matuszek_Munson_2015, Liang_Li_Zheng_Lim_Salakhutdinov_Morency_2020, Lloyd_2018, Luccioni_Corry_Sridharan_Ananny_Schultz_Crawford_2022, Paullada_Raji_Bender_Denton_Hanna_2021, Savoldi_Gaido_Bentivogli_Negri_Turchi_2021, Sondergaard_Hansen_2018, Sweeney_2013, tomalin2021practical, vanEs_2021, Wang_Barocas_Laird_Wallach_2022, Weidinger2022, Yee_Tantipongpipat_Mishra_2021, Zhao_Wang_Yatskar_Ordonez_Chang_2017, microsoft_2020}  \\ \midrule
Demeaning social groups & \cite{Abid_Farooqi_Zou_2021, Blodgett_Barocas_Daume_Wallach_2020, Dobbe_Dean_Gilbert_Kohli_2018, Jane_2018, Katzman_Barocas_Blodgett_Laird_Scheuerman_Wallach_2021, Kay_Matuszek_Munson_2015, Keyes_2018, Lloyd_2018, Monroe-White_2021, Paullada_Raji_Bender_Denton_Hanna_2021, samadi2018, Sweeney_2013, Thiago_Marcelo_Gomes_2021, Wang_Barocas_Laird_Wallach_2022, Weidinger2022, Yee_Tantipongpipat_Mishra_2021}  \\ \midrule
Erasing social groups & \cite{Devinney_2022, Field_Blodgett_Waseem_Tsvetkov_2021, Katzman_Barocas_Blodgett_Laird_Scheuerman_Wallach_2021, Wang_Barocas_Laird_Wallach_2022, Weidinger2022}  \\ \midrule
Alienating social groups & \cite{Kay_Matuszek_Munson_2015, Wang_Barocas_Laird_Wallach_2022}  \\ \midrule
Denying opportunity to self-identify / non-consensual representations & \cite{Chancellor_2019, Devinney_2022, Katzman_Barocas_Blodgett_Laird_Scheuerman_Wallach_2021, Paullada_Raji_Bender_Denton_Hanna_2021, Wang_Barocas_Laird_Wallach_2022, Wang_Ramaswamy_Russakovsky_2022, Raji_Gebru_Mitchell_Buolamwini_Lee_Denton_2020}  \\ \midrule
Reifying essentialist social categories & \cite{Dobbe_Dean_Gilbert_Kohli_2018, Hanna_Denton_Smart_Smith-Loud_2020, Hoffmann_2021, Jane_2018, Katzman_Barocas_Blodgett_Laird_Scheuerman_Wallach_2021, Keyes_2018, Monroe-White_2021, phan2019amazon, Raji_Gebru_Mitchell_Buolamwini_Lee_Denton_2020, Sadowski_Selinger_2014, Sambasivan_Arnesen_Hutchinson_Doshi_Prabhakaran_2021, Spiel2019, Wang_Barocas_Laird_Wallach_2022, Welbl_2021} \\ \hline
\end{longtable}
\end{center}

\begin{center}
\begin{longtable}{p{5cm}p{8cm}}
\caption{Allocative harms described in data sources.}
\label{allocativesources}\\
\toprule
Sub-type & References  \\ \midrule
Allocative harms (generally) & \cite{Angwin_Parris_2016, Bailey_Burkell_Dunn_Gosse_Steeves_2021, Balayn_Lofi_Houben_2021, Bandy2021, barocas-hardt-narayanan, binns2021, Blodgett_Barocas_Daume_Wallach_2020, Castillo_2019, cave2019bridging, corry2021problem, Davis_Williams_Yang_2021, Devinney_2022, Dev_Monajatipoor_Ovalle_Subramonian_Phillips_Chang_2021, Dobbe_Dean_Gilbert_Kohli_2018, Ekstrand_Das_Burke_Diaz_2022, Field_Blodgett_Waseem_Tsvetkov_2021, galaz2021artificial, galaz2021machine, Hoffmann_2021, Holstein_2019, Jacobs_2021, Jane_2018, Kaminski_Malgieri_2020, Kapania_Siy_Clapper_Sp_Sambasivan_2022, Knox_2019, Lloyd_2018, Luccioni_Corry_Sridharan_Ananny_Schultz_Crawford_2022, Mannes_2020, Markl_2022, Mashhadi_Zolyomi_Quedado_2022, Onuhoha, Ramesh_Kameswaran_Wang_Sambasivan_2022, Richardson_Gilbert_2021, Savoldi_Gaido_Bentivogli_Negri_Turchi_2021, Singh_Joachims_2018, Sun_Asudeh_Jagadish_Howe_Stoyanovich_2019, Suresh_Guttag_2021, Tufekci_Rit_Adam_Kramer_Guillory_Hancock, vanEs_2021, Weidinger2022, Weinberg_2022, Wu_Mitra_Ma_Diaz_Liu_2022, Yee_Tantipongpipat_Mishra_2021, Zajko_2022, rekabsaz2021, Metcalf_Moss_Watkins_Singh_Elish_2021} \\ \midrule
Opportunity loss & {Education discrimination}: ~\cite{Altman_Wood_Vayena_2018, Ehsan_Singh_Metcalf_Riedl_2022, Karumbaiah_Brooks_2021, Mashhadi_Zolyomi_Quedado_2022, microsoft_2020, Monroe-White_2021}; {Inequitable access to information/resources needed to participate in society}: \cite{cave2019bridging, Costanza-Chock_Raji_Buolamwini_2022, Kapania_Siy_Clapper_Sp_Sambasivan_2022, Markl_2022, Obermeyer_2019, Redden_Brand_2017}; {Housing discrimination}: ~\cite{Angwin_Parris_2016, Mashhadi_Zolyomi_Quedado_2022, Redden_Brand_2017, vanEs_2021, microsoft_2020} \\ \midrule

Economic loss & {Credit discrimination} \cite{Bandy2021, Jane_2018, Kapania_Siy_Clapper_Sp_Sambasivan_2022, Sambasivan_Arnesen_Hutchinson_Doshi_Prabhakaran_2021, Mannes_2020, Markl_2022, microsoft_2020, Monroe-White_2021, Redden_Brand_2017, Sambasivan_Arnesen_Hutchinson_Doshi_Prabhakaran_2021}; {Demonetization} \cite{Caplan_Gillespie_2020}; {Employment discrimination} \cite{Altman_Wood_Vayena_2018, DeVos_Dhabalia_Shen_Holstein_Eslami_2022, Jacobs_2021, koenecke2020racial, Krafft_2021, Lloyd_2018, microsoft_2020, Sambasivan_Arnesen_Hutchinson_Doshi_Prabhakaran_2021, Yee_Tantipongpipat_Mishra_2021}; {Financial injuries} \cite{Altman_Wood_Vayena_2018, Avila_2018, Dobbe_Krendl_Gilbert_Mintz_2021, Kapania_Siy_Clapper_Sp_Sambasivan_2022, Sambasivan_Arnesen_Hutchinson_Doshi_Prabhakaran_2021, Ramesh_Kameswaran_Wang_Sambasivan_2022, CSETTaxonomy, Metcalf_Moss_Watkins_Singh_Elish_2021}; {Insurance discrimination} \cite{Costanza-Chock_Raji_Buolamwini_2022, microsoft_2020}; {Loss of job opportunities} \cite{Altman_Wood_Vayena_2018, Krafft_2021, Mannes_2020, Wu_Mitra_Ma_Diaz_Liu_2022, Yee_Tantipongpipat_Mishra_2021}; {Price discrimination} \cite{Bandy2021, Chen_Mislove_Wilson_2016, microsoft_2020, Obermeyer_2019, Pandey_Caliskan_2021}\\ \hline
\end{longtable}
\end{center}

\begin{center}
\begin{longtable}{{p{5cm}p{8cm}}}
\caption{Quality-of-service harms described in data sources.}
\label{qosdatasources}\\
\toprule
Sub-type & References  \\ \midrule
Quality-of-service harms (generally) & 
\cite{binns2021,Buolamwini_Friedler_Wilson,DeVries_2019,Ekstrand_Das_Burke_Diaz_2022, joyce2021toward,Kaminski_Malgieri_2020, koenecke2020racial, Markl_2022, mengesha2021don, Obermeyer_2019, Raz_2021, Suresh_Guttag_2021, Rincon_Keyes_Cath_2021, Sambasivan_Arnesen_Hutchinson_Doshi_Prabhakaran_2021, Weidinger2022} \\ \midrule

Alienation & \cite{Bennett_Gleason_Scheuerman_Bigham_Guo_To_2021, Bivens_Haimson_2016, Blodgett_Barocas_Daume_Wallach_2020, Keyes_2018, Mannes_2020, mengesha2021don, Rincon_Keyes_Cath_2021, Weidinger2022} \\ \midrule

Increased labor & 
\cite{Bennett_Gleason_Scheuerman_Bigham_Guo_To_2021, Blodgett_Barocas_Daume_Wallach_2020, DeVos_Dhabalia_Shen_Holstein_Eslami_2022, koenecke2020racial, mengesha2021don} \\ \midrule
Service loss & {Algorithmic invisibility:} ~\cite{DeVries_2019, Duffy_Meisner_2022, Sambasivan_Arnesen_Hutchinson_Doshi_Prabhakaran_2021, Tatman_2017}; Degraded performance: ~\cite{aksenova-etal-2021-might,DeVries_2019,vanEs_2021,galaz2021machine, Hoffmann_2021, koenecke2020racial, Liao_2015, mengesha2021don, Obermeyer_2019, Tatman_2017} \\ \hline
\end{longtable}
\end{center}

\newpage
\begin{longtable}{{p{5cm}p{8.5cm}}}
\caption{Interpersonal harms described in data sources.}
\label{interpersonalsources}\\
\toprule
Sub-type & References  \\ \midrule
Loss of agency / Social control & Agency loss / Social control (generally): ~\cite{Dean_Gilbert_Lambert_Zick_2021, McGlynn_Rackley_2017,  Malik_Viljanen_Lepinkainen_Alvesalo-Kuusi_Others, Mann_Matzner_2019, Keyes_2018, Wang_2020,Agrafiotis_Nurse_Goldsmith_Creese_Upton_2018, Smuha_2021a, Karizat_2021, Andalibi_Garcia_2021, Skirpan_Fiesler_2018, Lustig_Konrad_Brubaker_2022, Bandy2021, Tufekci_Rit_Adam_Kramer_Guillory_Hancock, Weidinger2022, Thiago_Marcelo_Gomes_2021, Mohamed_Png_Isaac_2020, microsoft_2020, Bailey_Burkell_Dunn_Gosse_Steeves_2021, Birhane_Prabhu_Kahembwe_2021, Wang_Zhao_Van_Kleek_Shadbolt_2022, Moss_2021}; Algorithmically-informed identity change: ~\cite{Karizat_2021}\\ \midrule

Technology-facilitated violence & Technology-facilitated violence (generally): ~\cite{Brown_Sanci_Hegarty_2021, Freed_Palmer_Minchala_Levy_Ristenpart_Dell_2018, Henry_Flynn_Powell_2020, Bailey_Henry_Flynn_2021, Dev_Monajatipoor_Ovalle_Subramonian_Phillips_Chang_2021, Keyes_2018, Holstein_2019, Alkhatib2021, Scheuerman_Branham_Hamidi_2018, Wang_Zhao_Van_Kleek_Shadbolt_2022, Moss_2021};
Coercive control, or intimate partner violence: ~\cite{Dragiewicz_2018, Henry_Flynn_Powell_2020}; Inciting or enabling offline violence: ~\cite{Moss_2021, Tufekci_Rit_Adam_Kramer_Guillory_Hancock}; Online abuse (e.g., bullying, deadnaming, doxxing, trolling, hateful or toxic language): ~\cite{Maity_Chakraborty_Goyal_Mukherjee_2018, Vitak_Chadha_Steiner_Ashktorab_2017, Sheth_Shalin_Kursuncu_2021, Guberman_Schmitz_Hemphill_2016, Slonje_Smith_Frisen_2013, Ayodeji_Olamijuwon_Kokomma_Onyemelukwe_Gboyega_2021, Douglas_2016, Freed_Palmer_Minchala_Levy_Ristenpart_Dell_2018, Scheuerman_Jiang_Fiesler_Brubaker_2021, Ramesh_Kameswaran_Wang_Sambasivan_2022, Lloyd_2018, Feder_Cooper_Moss_Laufer_Nissenbaum_2022, brundage2018malicious, Scheuerman_Branham_Hamidi_2018, Sambasivan_Arnesen_Hutchinson_Doshi_Prabhakaran_2021, modei_Olah_Steinhardt_Christiano_Schulman_Mane_2016, Wang_Zhao_Van_Kleek_Shadbolt_2022}; Online sexual harassment (e.g., image-based abuse, cyberstalking, sexual harassment, sextortion): ~\cite{Ayodeji_Olamijuwon_Kokomma_Onyemelukwe_Gboyega_2021, Douglas_2016, Freed_Palmer_Minchala_Levy_Ristenpart_Dell_2018, Dragiewicz_2018, Henry_Flynn_Powell_2020, Ramesh_Kameswaran_Wang_Sambasivan_2022, Bandy2021, Altman_Wood_Vayena_2018, McGlynn_Rackley_2017, Sambasivan_Arnesen_Hutchinson_Doshi_Prabhakaran_2021, Henry_Flynn_Powell_2020, Bailey_Burkell_Dunn_Gosse_Steeves_2021} \\ \midrule

Diminished health and well-being & 
{Behavioral manipulation:} ~\cite{Karizat_2021, microsoft_2020}; Emotional harms (e.g., dignity loss, invalidation, misgendering): ~\cite{Bengio_Beygelzimer_Crawford_Fromer_Gabriel_Levendowski_Raji_Ranzato_2022, Wardle_and_Derakhshan_2017, Cambre_Kulkarni_2019, Karizat_2021, McGlynn_Rackley_2017, Agrafiotis_2016, Redden_Brand_2017, Scheuerman_Branham_Hamidi_2018, Vitak_Chadha_Steiner_Ashktorab_2017, Brown_Sanci_Hegarty_2021, Jane_2018, Mannes_2020, Dev_Monajatipoor_Ovalle_Subramonian_Phillips_Chang_2021, Keyes_2018, Thiago_Marcelo_Gomes_2021, Welbl_2021, Andalibi_Garcia_2021, Weidinger2022, Bandy2021, Feder_Cooper_Moss_Laufer_Nissenbaum_2022, brundage2018malicious, microsoft_2020, CSETTaxonomy, Wang_2020}; Physical harms: ~\cite{Bengio_Beygelzimer_Crawford_Fromer_Gabriel_Levendowski_Raji_Ranzato_2022, Wardle_and_Derakhshan_2017, Cambre_Kulkarni_2019, Karizat_2021, McGlynn_Rackley_2017, Agrafiotis_2016, Redden_Brand_2017, Mannes_2020, Scheuerman_Branham_Hamidi_2018, Vitak_Chadha_Steiner_Ashktorab_2017, Brown_Sanci_Hegarty_2021, Douglas_2016, Bennett_Gleason_Scheuerman_Bigham_Guo_To_2021, Scheuerman_Jiang_Fiesler_Brubaker_2021, Pendse2022, Ramesh_Kameswaran_Wang_Sambasivan_2022, DeVos_Dhabalia_Shen_Holstein_Eslami_2022, microsoft_2020, CSETTaxonomy, Wang_Ramaswamy_Russakovsky_2022}; Reputational harms: ~\cite{Redden_Brand_2017, Bennett_Gleason_Scheuerman_Bigham_Guo_To_2021, Png_2022, CSETTaxonomy, Metcalf_Moss_Watkins_Singh_Elish_2021, Moss_2021, Agrafiotis_2016, Bailey_Burkell_Dunn_Gosse_Steeves_2021, Sanchez2021, Hutchinson2020socialbiases} \\ \midrule
Privacy violations & {Privacy violations (generally):} ~\cite{Bengio_Beygelzimer_Crawford_Fromer_Gabriel_Levendowski_Raji_Ranzato_2022, McGlynn_Rackley_2017, Redden_Brand_2017, Mannes_2020, Welbl_2021, Ehsan_Singh_Metcalf_Riedl_2022, Chancellor_2019, binns2021, Formosa_Wilson_Richards_2021, Chi_Lurie_Mulligan, Ekstrand_Das_Burke_Diaz_2022, Png_2022, Kaminski_Malgieri_2020, Weidinger2022, Slupska_Dawson_Duckworth_Ma_Neff_2021, Ramesh_Kameswaran_Wang_Sambasivan_2022, corry2021problem, Tufekci_Rit_Adam_Kramer_Guillory_Hancock, Birhane_2021, Dobbe_Krendl_Gilbert_Mintz_2021, Feder_Cooper_Moss_Laufer_Nissenbaum_2022, microsoft_2020, Moss_2021, Metcalf_Moss_Watkins_Singh_Elish_2021, Raji_Gebru_Mitchell_Buolamwini_Lee_Denton_2020, Bailey_Burkell_Dunn_Gosse_Steeves_2021, Wang_Zhao_Van_Kleek_Shadbolt_2022}; Algorithmic profiling: ~\cite{Mohamed_Png_Isaac_2020, Sambasivan_Arnesen_Hutchinson_Doshi_Prabhakaran_2021, Redden_Brand_2017, Mann_Matzner_2019, Monroe-White_2021}; Feelings of surveillance, or loss of desired anonymity: ~\cite{Rincon_Keyes_Cath_2021, Mann_Matzner_2019, Ehsan_Singh_Metcalf_Riedl_2022, Monroe-White_2021, Costanza-Chock_Raji_Buolamwini_2022, Krafft_2021, Markl_2022, Skirpan_Fiesler_2018, Katell_Young_Dailey_Herman_Guetler_Tam_Bintz_Raz_Krafft_2020, Slupska_Dawson_Duckworth_Ma_Neff_2021, van_der_Sloot_van_Schendel_2021}; Loss of right to be forgotten: ~\cite{Altman_Wood_Vayena_2018, Wang_Zhao_Van_Kleek_Shadbolt_2022}; Non-consensual data collection: ~\cite{Kapania_Siy_Clapper_Sp_Sambasivan_2022}; Privacy attacks (e.g., identity theft, doxxing): ~\cite{Redden_Brand_2017, Douglas_2016, Bandy2021} \\ \hline
\end{longtable}
%\end{center}

\newpage
\begin{center}
\begin{longtable}{{p{5cm}p{8cm}}}
\caption{Social system harms described in data sources.}
\label{societaldatasources}\\
\toprule
Sub-type & References  \\ \midrule

Social system harms (generally) & 
{Societal harms (generally):} \cite{Agrafiotis_Nurse_Goldsmith_Creese_Upton_2018, Agrafiotis_2016, Bengio_Beygelzimer_Crawford_Fromer_Gabriel_Levendowski_Raji_Ranzato_2022, microsoft_2020, Redden_Brand_2017, van_der_Sloot_van_Schendel_2021, CSETTaxonomy, Wardle_and_Derakhshan_2017}; Amplifying existing power disparities: \cite{Altman_Wood_Vayena_2018, Avila_2018, Bailey_Burkell_Dunn_Gosse_Steeves_2021, Bandy2021, Barabas_Doyle, barocas-hardt-narayanan, BarocasSelbst_2016, Bedford_Mann_Foth_Walters_2022, Benjamin_2019, Bennett_Gleason_Scheuerman_Bigham_Guo_To_2021, binns2021, Birhane_2021, Blodgett_Barocas_Daume_Wallach_2020, Buolamwini_Friedler_Wilson, Chi_Lurie_Mulligan, corry2021problem, Costanza-Chock_Raji_Buolamwini_2022, Davis_Williams_Yang_2021, Chancellor_2019, Dev_Monajatipoor_Ovalle_Subramonian_Phillips_Chang_2021, Dobbe_Krendl_Gilbert_Mintz_2021, Dosono_Semaan_2020, Dragiewicz_2018, Ehsan_Singh_Metcalf_Riedl_2022, Ekstrand_Das_Burke_Diaz_2022, Fazelpour_Lipton_2020, Field_Blodgett_Waseem_Tsvetkov_2021, Hendricks_Burns_Saenko_Darrell_Rohrbach_2018, Hoffmann_2021, Hutchinson_Prabhakaran_Denton_2020, Hutchinson2020socialbiases, Jacobs_2021, joyce2021toward, Karizat_2021, Karumbaiah_Brooks_2021, Katell_Young_Dailey_Herman_Guetler_Tam_Bintz_Raz_Krafft_2020, Knox_2019, Lloyd_2018, Malik_Viljanen_Lepinkainen_Alvesalo-Kuusi_Others, Mann_Matzner_2019, Markl_2022, McGlynn_Rackley_2017, Mohamed_Png_Isaac_2020, Moss_2021, Nedzhvetskaya_Tan_2021, Raji_Gebru_Mitchell_Buolamwini_Lee_Denton_2020, Ramesh_Kameswaran_Wang_Sambasivan_2022, Richardson_Gilbert_2021, Sambasivan_Arnesen_Hutchinson_Doshi_Prabhakaran_2021, Savoldi_Gaido_Bentivogli_Negri_Turchi_2021, Scheuerman_Jiang_Fiesler_Brubaker_2021, Shen_2021, Sloane_Moss_Awomolo_Forlano_2020, Smuha_2021b, Smuha_2021c, Suresh_Guttag_2021, Thiago_Marcelo_Gomes_2021, vanEs_2021, Weidinger2022, Weinberg_2022, Zajko_2022, Zhao_Wang_Yatskar_Ordonez_Chang_2017, Wang_2020, Metcalf_Moss_Watkins_Singh_Elish_2021} \\ \midrule

Information harms & Information harms (generally): \cite{Altman_Wood_Vayena_2018, CSETTaxonomy, Wardle_and_Derakhshan_2017}; Disinformation: \cite{Ekstrand_Das_Burke_Diaz_2022, janzen2022cognitive, Wardle_and_Derakhshan_2017, Wardle_Singerman_2021}; Distortion of reality: \cite{Altman_Wood_Vayena_2018, Bandy2021, Dosono_Semaan_2020, microsoft_2020}; Information asymmetries: \cite{Caplan_Gillespie_2020}; Malinformation: \cite{janzen2022cognitive, Wardle_and_Derakhshan_2017}; Misinformation: \cite{modei_Olah_Steinhardt_Christiano_Schulman_Mane_2016, Blodgett_Barocas_Daume_Wallach_2020, brundage2018malicious, Chancellor_2019, Ekstrand_Das_Burke_Diaz_2022, Katell_Young_Dailey_Herman_Guetler_Tam_Bintz_Raz_Krafft_2020, microsoft_2020, Neumann_De-Arteaga_Fazelpour_2022, Pendse2022, Smuha_2021c, Southwell_Brennen_Paquin_Boudewyns_Zeng_2022, Tran_Valecha_Rad_Rao_2020, Treen_Williams_ONeill_2020, Wardle_and_Derakhshan_2017, Wardle_Singerman_2021, Weidinger2022, Weinberg_2022, Wright_Williams_Elizarova_Dahne_Bian_Zhao_Tan_2021}; Subjugating and reshaping knowledge: \cite{DeVos_Dhabalia_Shen_Holstein_Eslami_2022, Sadowski_Selinger_2014, Singh_Joachims_2018}\\ \midrule

Cultural harms & Cultural harms (generally):
~\cite{DeVos_Dhabalia_Shen_Holstein_Eslami_2022, Dobbe_Dean_Gilbert_Kohli_2018, Irani_Vertesi_Dourish_Philip_Grinter_2010, Malik_Viljanen_Lepinkainen_Alvesalo-Kuusi_Others}; 
Cultural hegemony: ~\cite{Docherty_Biega_2022, Dosono_Semaan_2020}; Deteriorating social bonds: ~\cite{McGlynn_Rackley_2017}; Erasure: ~\cite{Devinney_2022, DeVos_Dhabalia_Shen_Holstein_Eslami_2022, Dosono_Semaan_2020, Keyes_2018, Sambasivan_Arnesen_Hutchinson_Doshi_Prabhakaran_2021}; Misinformation about social groups: ~\cite{Dosono_Semaan_2020, Sambasivan_Arnesen_Hutchinson_Doshi_Prabhakaran_2021} \\ \midrule

Political and civic harms & Political and civic harms (generally): ~\cite{Malik_Viljanen_Lepinkainen_Alvesalo-Kuusi_Others, Redden_Brand_2017, Satra_2020, Satra_2021, CSETTaxonomy}; Erosion of democracy (e.g., election interference, censorship, harm to civil liberties): ~\cite{Birhane_2021, corry2021problem, Green_Viljoen_2020, Lloyd_2018, microsoft_2020, Satra_2020, Satra_2021, Skirpan_Fiesler_2018, Smuha_2021b, Tufekci_Rit_Adam_Kramer_Guillory_Hancock, Moss_2021}; Human rights violations: \cite{Agrafiotis_2016, microsoft_2020, Moss_2021, Satra_2021, Sambasivan_Arnesen_Hutchinson_Doshi_Prabhakaran_2021, Yeung_Howes_Pogrebna}; Legal system harms (e.g., wrongful arrest, court transcription errors, unreasonable searches): ~\cite{modei_Olah_Steinhardt_Christiano_Schulman_Mane_2016, brundage2018malicious, Costanza-Chock_Raji_Buolamwini_2022, Dobbe_Dean_Gilbert_Kohli_2018, Feder_Cooper_Moss_Laufer_Nissenbaum_2022, koenecke2020racial, Mannes_2020, Redden_Brand_2017, Tufekci_Rit_Adam_Kramer_Guillory_Hancock, Moss_2021}; Nation destabilization (e.g., social polarization, loss of legitimacy): ~\cite{Agrafiotis_Nurse_Goldsmith_Creese_Upton_2018, Mohamed_Png_Isaac_2020, Satra_2020, Skirpan_Fiesler_2018, Smuha_2021b} \\ \midrule

Macro socio-economic harms & Macro socio-economic harms (generally): \cite{Agrafiotis_2016, Malik_Viljanen_Lepinkainen_Alvesalo-Kuusi_Others, Png_2022, Weidinger2022}; Algorithmic flash crashes: \cite{Agrafiotis_2016, Malik_Viljanen_Lepinkainen_Alvesalo-Kuusi_Others, Mohamed_Png_Isaac_2020}; Data harms: \cite{Mohamed_Png_Isaac_2020}; Digital divides: \cite{Ayodeji_Olamijuwon_Kokomma_Onyemelukwe_Gboyega_2021, Field_Blodgett_Waseem_Tsvetkov_2021, Irani_Vertesi_Dourish_Philip_Grinter_2010, microsoft_2020, Wang_Zhao_Van_Kleek_Shadbolt_2022, modei_Olah_Steinhardt_Christiano_Schulman_Mane_2016, galaz2021artificial};
Labor exploitation: \cite{Docherty_Biega_2022, microsoft_2020, Mohamed_Png_Isaac_2020};
Technological unemployment (e.g., professional displacement, disruption to livelihood, automation of tasks, devaluation of human expertise): \cite{Bengio_Beygelzimer_Crawford_Fromer_Gabriel_Levendowski_Raji_Ranzato_2022, cave2019bridging, joyce2021toward, microsoft_2020, Png_2022}; Worsening worker conditions: \cite{Bengio_Beygelzimer_Crawford_Fromer_Gabriel_Levendowski_Raji_Ranzato_2022}\\ \midrule

Environmental harms & Environmental harms: Ecological harms/depletion of natural resources: \cite{Bandy2021, Bedford_Mann_Foth_Walters_2022, microsoft_2020, Mohamed_Png_Isaac_2020, Png_2022, Smuha_2021c, Weidinger2022, Welbl_2021, Moss_2021, galaz2021machine}; 
Damage to built environment: \cite{Bandy2021, Mannes_2020, Smuha_2021b, CSETTaxonomy}; Injury to animals: \cite{Dean_Gilbert_Lambert_Zick_2021} \\ \hline
\end{longtable}
\end{center}
